# Supplementary material for: Supercurrent in a double quantum dot
Source: arXiv:1808.05837 ancillary file (2020-04-27)
Supplement: Supplementary file 1 [file Supplement_Estrada2018.pdf]

# Supplemental Material: Supercurrent in a double quantum dot

J. C. Estrada Saldaña[1], A. Vekris[1], G. Steffensen[1], R. Žitko[2], P. Krogstrup[1], J. Paaske[1], K. Grove-Rasmussen[1], and J. Nygård[1]
[1] *Center for Quantum Devices, Niels Bohr Institute, University of Copenhagen, 2100 Copenhagen, Denmark and*
[2] *Jožef Stefan Institute, Jamova 39, Ljubljana, Slovenia*
*Faculty of Mathematics and Physics, University of Ljubljana, Jadranska 19, Ljubljana, Slovenia*

## CONTENTS

I. Extraction of $U$ and $\Delta E$ of each dot 2

II. Direct extraction of the switching current 3

III. Fitting method 4

IV. Yu-Shiba-Rusinov subgap states 4

V. Magnetic field dependence of subgap features 6

VI. (-1,1) and (1,3) charge sectors 7

VII. Spectroscopy of the convoluted gap and temperature dependence 7

VIII. Theoretical models for supercurrent 10
A. Perturbation theory 10
B. Zero-Bandwidth approximation 13

IX. Numerical renormalization group 15
A. Γ-dependence of the Josephson current 16
B. NRG results for the S-DQD-S problem 17

X. $I_c$ crossings at the $0-\pi$ transition 19

References 20

Here we show our fitting methodology, direct measurements of the switching current consistent with the qualitative behavior of fitted critical current, additional supercurrent data at other charge states, a spectroscopy of the subgap states consistent with our interpretation of the supercurrent data, and our theory models.

## I. EXTRACTION OF $U$ AND $\Delta E$ OF EACH DOT

Figure S1a shows a zoomed-out version of the colormap of linear conductance, $G$, of Fig. 2 of the main text, depicting adjacent charge states to the ones showed there. In this map, the parity-change lines belonging to each of the dots exhibit an alternating spacing pattern, typical of shell filling of quantum dot levels [S1]. It is this pattern that allowed us to define the (1,1) charge sector, which corresponds to the pair of DQD shells that was studied extensively on the main article. Using that charge sector as reference, we labeled other close-by charge states as (-1,1) and (1,3). DQD shells corresponding to charge states (1,1) and (1,3) appear to have similar couplings to the leads given their similar conductance pattern. Moreover, the critical current, shown in a section below, behaves the same as in the example shown in the main text. On the other hand, the (-1,1) charge sector has noticeably lower conductance, which is most probably due to an influence of $V_{gL}$ on $\Gamma_L$ -i.e., lower $V_{gL}$ decreases $\Gamma_L$. The critical current in this DQD shell was much smaller, but the overall behavior described in the main text also applied here, as shown later.

The observed shell-filling pattern supports our treatment of the two serial quantum dots as two *single* orbitals in series. A more quantitative analysis shows that the level spacing, extracted by converting the spacings between adjacent charge transitions to energy with the aid of the lever-arm parameters of each dot, is significant compared to the charging energy of the each dot. We extracted $U_R \approx 1.75$ meV, $\Delta E_R \approx 1.76$ meV, for the right dot and $U_L \approx 2.1$ meV, $\Delta E_L \approx 1.64$ meV, for the left one. These values are only approximate, since $U$ is influenced by the couplings $\Gamma_{L,R}$ and superconductivity. To complement and refine these estimations, we also measured $U$ and $\Delta E$ using Coulomb diamonds spectroscopy which is illustrated in Figure S1b,c. We obtained $U_R \approx 1.62$ meV and $\Delta E_R \approx 1.75$ meV for the right dot and $U_L \approx 1.85$ meV for the left one. The two estimations of $U$ show a negligible difference in the extracted values. $\Delta E_L$ could not be measured using bias spectroscopy, since there was no clear evidence on the plot of an excited state. Hence, we only provide the value extracted from Fig. S1a. Since $U \sim \Delta E$, the two dots can be treated as single orbitals [S2], as assumed in our model.

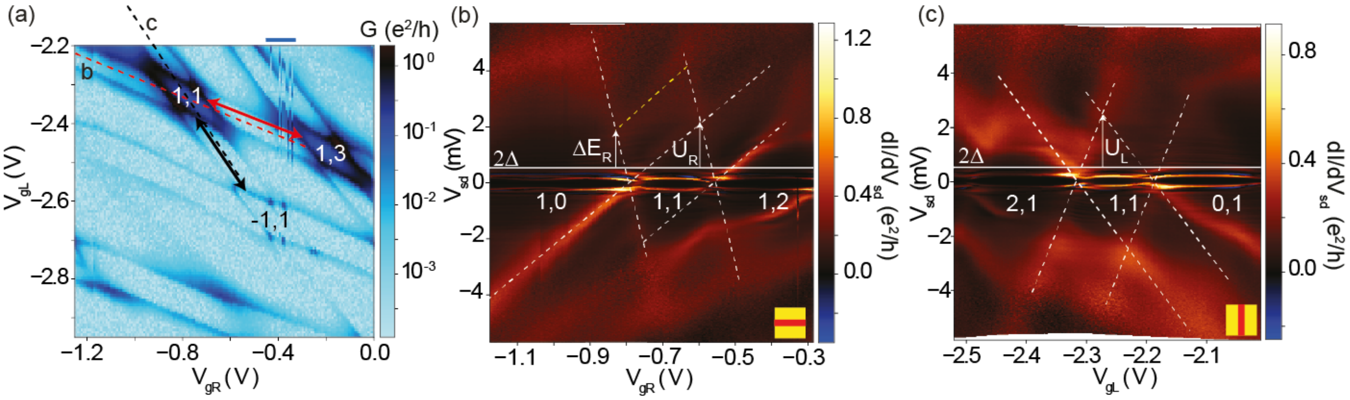


FIG. S1. (a) Charge stability diagram showing three different DQD shells. A zoom-in of the nine charge states (pair of DQD shells) surrounding -and including- sector (1,1) was shown in Fig. 2 of the main article. Dashed lines indicate the cut directions of panels (b) (red) and (c) (black). Arrowhead lines indicate $U_i + \Delta E_i$ of the left (i=L, black) and the right (i=R,red) dot respectively. A horizontal blue line on the top indicates a $V_{gR}$ region of reproducible charge instability, due to uncontrolled charge trapping and discharging in the electrostatic environment of the device. This causes an apparent doubling or displacement of features in the charge states (1,3) and (-1,1) in this map. (b) Large-bias spectroscopy of right-dot Coulomb diamonds, highlighted by white dashed lines to guide the eye. The white horizontal line is a reference for the superconducting gap $2\Delta = 0.53$ meV -not visible in this regime [S3]-, taken from the data at lower coupling shown in Fig. S6. From the graph we could extract the charging energy of the right dot, $U_R$, as well as the level spacing, $\Delta E_R$, by measuring the distance to the first excited state (yellow dashed line). The lever-arm parameter, $\alpha_R = 0.009$, was found using the white dashed lines as reference. (c) High-bias spectroscopy of left-dot Coulomb diamonds. The charging energy of the left dot, $U_L$, was extracted with the same graphical method. The lever-arm parameter of this dot was estimated at $\alpha_L = 0.02$.

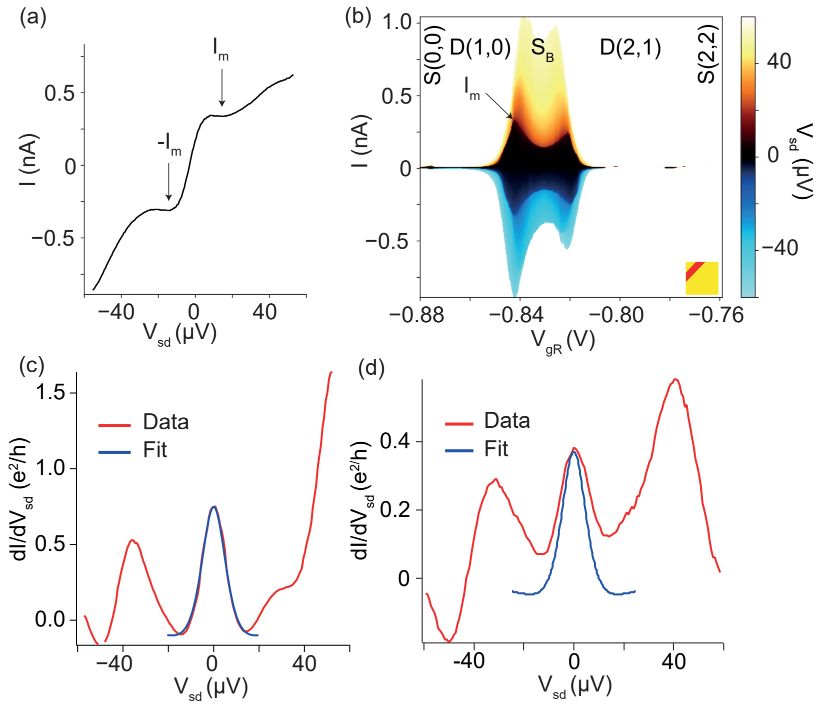


FIG. S2. (a) Example of an I-V curve exhibiting an overdamped supercurrent. The current at $|I| < I_m$ is symmetric with respect to zero as expected for this kind of junction, and appears at finite voltage due to thermal noise. This curve was taken at $V_{gR} = -0.84$ V from the colormap in the next panel. (b) Colormap of the applied source-drain voltage, $V_{sd}$, as a function of the measured current, $I$, and the plunger voltage. $I$ in this map was recorded in simultaneous with the differential conductance in the map of Fig. 5b of the main text. Therefore, the fitted $I_c$ in the inset of that plot can be compared to directly-measured $I_m$ shown here. Charge transitions obtained from that map are also indicated here for reference. The color scale has been adjusted to highlight the dissipative supercurrent branch between $\pm I_m$ (in black), but it is not saturated. White regions indicate absence of data due to small current. Note that the fitted $I_c$ displayed in Fig. 5b of the main text is around six times larger than $I_m$, revealing a strong reduction of the switching current by thermal noise, as observed before in S-N-S junctions [S4]. (c) Example of a fit to a supercurrent zero-bias peak done to extract the critical current of the junction. (d) Example of an *unreliable* fit due to crossing of a pair of subgap states at zero bias. Notice that, in contrast to a supercurrent peak, this type of crossing produces a peak asymmetric in $V_{sd}$ and noticeably wider, with a significant conductance background. The quality of the fit noticeably deteriorates in this case.

## II. DIRECT EXTRACTION OF THE SWITCHING CURRENT

In spite of thermal noise, it was possible to directly extract the switching current, $I_m$, of the overdamped Josephson junction, provided that it attained a large enough value. In order to obtain $I_m$ as well as the fitted $I_c$ value, we also recorded the current through the junction simultaneously with the $dI/dV_{sd}$ signal displayed in the maps of Figs. 3a-d, 4a,b, and 5a-d of the main text. Fig. S2a shows an I-V curve taken from the colormap in panel (b) at $V_{gR} = -0.84$ V. The map was composed by plotting the applied $V_{sd}$ as a function of the recorded current taken while measuring the colormap in Fig. 5b of the main text. In Fig. S2a, $I_m$ has been indicated by a black arrow. Note that due to thermal white noise the slope of the current reaches a finite value between $\pm I_m$ [S4–S7]. Importantly, in this range the current is symmetric with respect to zero as expected in an overdamped junction, with switching occurring symmetrically at $I_m$ and $-I_m$. In turn, the presence of subgap states distorts the current in the ohmic branch at $I > |I_m|$, rendering it non-symmetric with respect to zero. The negative differential conductance (NDC) that accompanies the zero-bias supercurrent peak observed in the maps of Figs. 3a-d, 4a,b, and 5a-d of the main text comes from the decrease in current when $I_m$ is reached.

Fig. S2b shows a $V_{sd}(V_{gR}, I)$ map (obtained as explained above) on which the gate-dependent switching current is pointed by an arrow. The color scale has been adjusted to show the supercurrent branch in black. Note that the supercurrent symmetry with respect to $I = 0$ is preserved in the whole gate range, indicating that the Josephson junction is overdamped regardless of the value of the supercurrent. Though $I_m$ recorded this way shows the same qualitative dependence in gate voltage between the D(1,0) and S(2,1) ground states as fitted $I_c$ in Fig. 5b of the main text, the ground state transitions given by the small discontinuity in $I_c$ at S(0,0) → D(1,0) and D(2,1) → S(2,2) are

not captured by $I_m$ extracted in this way. This occurs because at this points $I_m$ is too smeared and small to be detected, whereas the fit adequately extracts an $I_c$ from the still visible zero-bias peak in differential conductance.

## III. FITTING METHOD

When thermal fluctuations are important with respect to the Josephson energy, $E_J = \hbar I_c/(2e)$, an overdamped Josephson junction will show a dissipative supercurrent *peak* [S4–S6], whose I-V characteristic is given by Eq. S1, where $I_\alpha(x)$ is the modified Bessel function of complex order $\alpha$, $\eta(V_{sd}) = \hbar V_{sd}/(2eRk_BT)$, and $\beta = I_c\hbar/(2ek_BT)$ is the ratio between the Josephson energy and the thermal energy. This equation has been used to extract the critical current of quantum-dot Josephson junctions, provided that the current-phase relationship is approximated to that of a tunnel junction [S7–S9].

$$I(V_{sd}) = \frac{R_J}{R_J + R}\left(I_c Im\left[\frac{I_{1-i\eta(V_{sd})}(\beta)}{I_{-i\eta(V_{sd})}(\beta)}\right] + \frac{V_{sd}}{R_J}\right) \tag{S1}$$

To estimate whether the junction is overdamped or underdamped, we calculate the quality factor which is given by Eq. S2 (see Supplementary Information of Ref. [S10]).

$$Q = \frac{\sqrt{\hbar(C(1 + R/R_J) + C_J)/(2eI_c)}}{RC + \hbar/(2eI_cR_J)} \tag{S2}$$

We find that for the maximum observed supercurrent, $I_c \approx 2$ nA, the extracted value is $Q = 0.11$. $Q < 1$ is a signature that the junction is overdamped, which can also be verified by the symmetry of the measurements with respect to $V_{sd} = 0$. For smaller $I_c$, $Q$ becomes smaller. The capacitance of the junction, $C_J = 2.8$ aF, was estimated by modeling the InAs nanowire junction as a parallel plate capacitor. The sub-gap resistance of the junction $R_J = 1$ G$\Omega$, the thermal resistor $R = 3$ k$\Omega$, and the temperature $T = 80$ mK were extracted through the fitting procedure by initially keeping all four parameters free -including $I_c$-, checking for consistency across various gate values over a scale of two orders of magnitude in conductance. The last parameter, $C = 9$ pF, was estimated by modeling the capacitance of the leads through the backgate as a parallel plate capacitor.

To fit our data, we first subtracted the series resistance of the filters ($R_s = 8.24$ k$\Omega$) from the raw bias voltage $V_{sd} = V_{raw} - IR_s$, since the measurement was done in a two-terminal configuration. Fitting $I - V_{sd}$ or $dI/dV_{sd}$-$V_{sd}$ curves gave the same results, but to fit $dI/dV_{sd}$ curves we first subtracted the filters resistance from the differential conductance. Additionally, to fit $dI/dV_{sd}$-$V_{sd}$ traces we first derived analytically Eq. S1 with respect to $V_{sd}$.

The fit is remarkably robust. With one free parameter ($I_c$), keeping the others fixed at $T = 80$ mK, $R = 3$ k$\Omega$ and $R_J = 1$ G$\Omega$ [S11], it is possible to fit all the low-bias differential conductance data shown in this article and also in various regimes not shown here, including larger tunnel coupling and finite magnetic field. Fig. S2c shows an example of a fit done to a $dI/dV_{sd}$-$V_{sd}$ curve taken at $V_{gR} = -0.83$ V from the colormap in Fig. 3b of the main text. In this curve, surrounding the supercurrent-zero bias peak, a pair of subgap states are seen at $\pm 30\mu V$. To avoid these -when possible-, the fits were done between $V_{sd} = \pm 20\mu$V.

The fit only fails whenever subgap states cross zero-bias at a ground state transition (see next section), due to the presence of a subgap state-related zero-bias conductance peak. The width of the subgap-states peak is gate-dependent, and it is not generally symmetric with respect to zero-bias, in striking contrast to the supercurrent zero-bias peak, which eases its identification. An example of such a case is shown in Fig. S2d, which corresponds to a $dI/dV_{sd}$-$V_{sd}$ curve taken at $V_{gR} = -0.58$ V from the colormap in Fig. 3d of the main article, and the best possible fit to this curve using the derivative of Eq. S1, with $I_c$ as the only free parameter. Data points of unreliable fitting due to this reason were replaced by dashed lines in Figs. 3a-d, 4a,b, and 5a-d of the main text.

## IV. YU-SHIBA-RUSINOV SUBGAP STATES

In the limit of $U \gg \Delta$, quasiparticle excitations are energetically inexpensive. The effect of a singly-occupied quantum dot level on an adjacent superconductor is the breaking of Cooper pairs into quasiparticle excitations, which can reside within the superconducting gap occupying subgap states. These subgap states are named Yu-Shiba-Rusinov (YSR) states [S3]. In asymmetric S-QD-N and S-DQD-N devices, for which $\Gamma_S \gg \Gamma_N$, and in the limit when $\Gamma_S$ is small with respect to $U$, these states show a characteristic loop structure in the differential conductance, with crossings of the Fermi level at parity changes [S12–S17]. Furthermore, the differential conductance lacks the peaks of

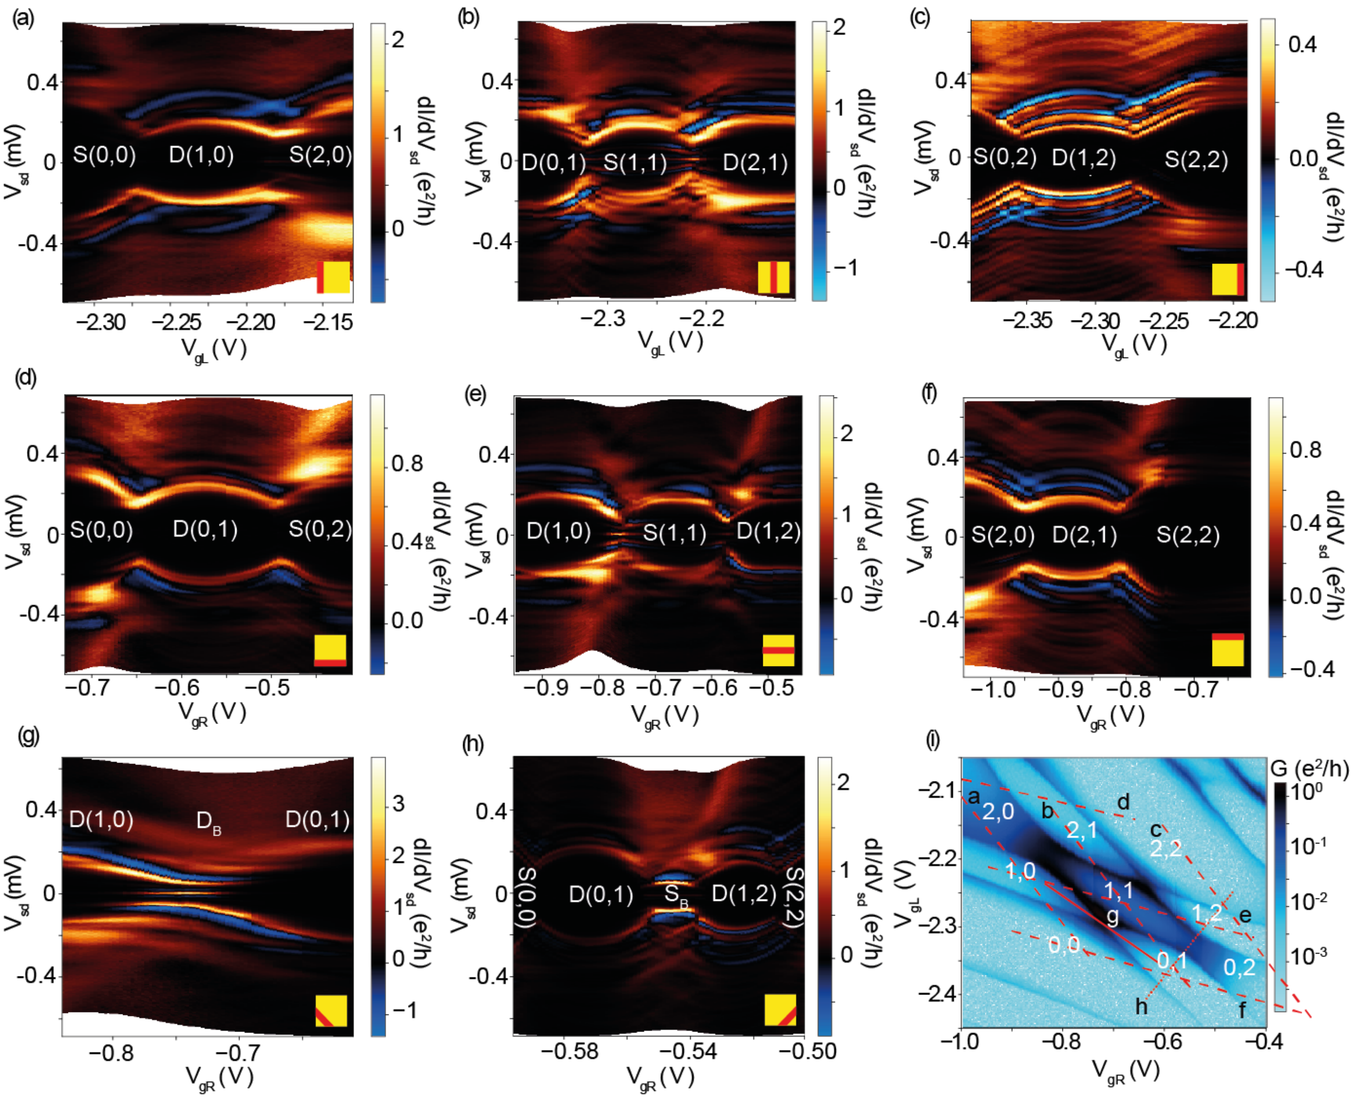


FIG. S3. (a-h) Differential conductance maps following the gate trajectories indicated in panel (i), depicting Yu-Shiba-Rusinov (YSR) subgap states seen at a larger bias window that the one shown in the main article. The ground state in each charge sector, as determined by the gate dependence of the supercurrent, is consistent with the gate dependence of the subgap states.

the continuum singularities [S3]. In asymmetric S-QD-S systems, pairs of YSR states are separated by $\Delta$ from $V_{sd}$=0, due to the presence of the superconducting gap in the lead with the lowest coupling to the dot, and are accompanied by negative differential conductance (NDC) [S18–S22].

Transport through an S-DQD-S system has recently been investigated, but the soft gap of the device resulted in an effective S-DQD-N spectroscopy, thus limiting the experimental precedence of this example for our case [S23]. In turn, available theoretical calculations only show spectral functions or energy level positions [S17], and not the expected differential conductance characteristic of the S-DQD-S system.

It is therefore unknown, both experimentally and theoretically, what the outcome of an spectroscopy of the subgap states of a hard-gapped genuine S-DQD-S system may be. In the limit of $t_d \to 0$, subgap states with energies $E_{bL}$ and $E_{bR}$ can be present in both leads, and these will probe each other as the bias voltage is swept. If the spectral weight of the continuum singularities is not negligible (i.e., $U \geqslant \Delta$), one can expect up to four peaks within the gap, by simple convolution of the density of states in the two leads. Moreover, more than one excitation can be present below the continuum, because the serial two-level system has more excitations than the single-level system [S17], thus increasing the number of peaks that one can expect in transport through the gap. For non-negligible $t_d$, a simple convolution method is in principle not enough to provide even the right qualitative picture. For strong $t_d$, higher-order coherent processes known as multiple Andreev reflections, present in the single dot system with strong symmetric coupling to the leads [S24], might occur, complicating the naive picture drawn above.

Our DQD device is in the limit of $U_L, U_R \gg \Delta$ in which YSR states are expected [S17], and their presence is confirmed by experiment. Figures S3a-f show line-cuts taken through the trajectories shown in Fig. S3g, which is the same $G$ map shown in Fig. 2 of the main article. These cuts are differential conductance maps taken at a larger $V_{sd}$ window than the supercurrent maps shown in the main article. Panels (a-c) show the dispersion of subgap states as a function of the occupation in the left dot, while keeping the occupation in the right dot fixed. In turn, panels (d-f) show this dispersion as a function of the occupation in the right dot, while keeping the occupation in the left dot fixed. These six maps exhibit the characteristic split-loop structure of pairs of YSR states being probed by a gapped spectra discussed above. Remarkably, the maps also show additional -though not exact- replicas of the lowest-lying pair of subgap states [S25]. In these maps, the apparent lowest-lying pair does not cross at $V_{sd}$=0 [S26], but does not cross either at $V_{sd} = \Delta = 0.265mV$, as one would expect from a decoupled superconductor lead probing a pair of subgap states in the other lead. Instead, the states cross at $V_{sd} \approx 0.1$ mV. This observation, together with their width -of about 10$\mu$V- and the fact that typically two to four of the lowest-lying pairs of peaks are followed by NDC, implies that the states are being probed by subgap peaks in the other lead, and not necessarily by decoupled continuum singularities.

Panel (g) probes the evolution of these subgap states in the detuning direction, following the continuous line in panel (i), with $D_B$ indicating the maximally-hybridized doublet bonding ground state at zero detuning. As detuning is increased either to the right or left of this state, the lowest lying pair of subgap states moves up in bias. This is consistent with the detuning modulation of $I_c$ observed in Fig. 4a of the main article. Moreover, the subgap states anticross at zero detuning -instead of making a split-loop-, indicating that the parity is constant across the whole map, which is again consistent with our interpretation of a constant doublet ground state as revealed by the gate dependence of $I_c$. This qualitative behavior was consistently observed for detuning line-cuts through the other three quadruple points (i.e., through the two $S_B$ and the remaining $D_B$ ground states). The lowest YSR states are asymmetric in bias, displaying a strong peak followed by NDC at positive bias in the D(1,0) sector, and a similar peak at negative bias in the D(0,1) sector. These states become symmetric only at zero detuning, indicating that their asymmetry is related to finite detuning.

Finally, panel (h) shows the evolution of the subgap states while shifting both orbitals with respect to the Fermi level while the orbitals remain aligned with each other, following the same gate trajectory as Fig. 5a of the main article. It is apparent from this map that the same kind of loops observed in panels (a-f) occur for the parity changes S(0,0)$\rightarrow$D(0,1) and D(1,2)$\rightarrow$S(2,2). However, the crossings which occur at the parity changes D(0,1)$\rightarrow S_B \rightarrow$D(1,2) are qualitatively different. In particular, the lowest-lying pair of subgap states at the $S_B$ sector are pushed towards zero bias, and exhibit little dispersion. This is consistent with relatively strong $I_c$ in this sector as shown in Fig. 5a of the main article.

Overall, the behavior of these YSR states corroborates the ground state transitions revealed by supercurrent discontinuities in the main text.

## V. MAGNETIC FIELD DEPENDENCE OF SUBGAP FEATURES

We also explored the dependence of subgap features on the magnetic field, $B$, with $B$ aligned parallel to the long axis of the nanowire. The goal of these measurements was to show magnetic tuning of $I_c$ and the related ground state of the system. Unfortunately, this was not possible, due to a crossing of subgap states with zero bias at $B = 0.16$ T, which obscured the $B$-dependence of the supercurrent zero-bias peak at larger field.

Figures S4a,b show the $B$ evolution of the subgap features taken at the center (red asterisks in panel (d)) of charge sectors (0,0) and (1,1), respectively. In both cases, subgap states rapidly converge at zero bias as $B$ is increased to $B = 0.16$ T (indicated by vertical black arrows). In sector (1,1), the supercurrent zero-bias peak remains visible until it is obscured by these states. At larger $B$ the subgap peaks seem to re-open, but a clear supercurrent zero-bias peak cannot be discerned anymore. In sector (0,0), for which supercurrent is absent due to Coulomb blockade, the conductance at and around zero-bias increases to a finite value above the same $B = 0.16$ T, due to a qualitatively similar crossing of the lowest-lying subgap states.

The $B$ evolution of the linear conductance, $G$, which probes parity peaks (horizontal red arrows) of the left quantum dot versus $B$, is depicted in Fig. S4c, corresponding to a line-cut through the dashed line in panel (d). $G$ shows a significant increase at $B > 0.16$ T (indicated by a vertical black arrow), particularly at the Coulomb blockaded regions between two pairs of parity peaks. Moreover, the peaks themselves become broader above this field. These two observations are consistent with broad and multiple subgap states crossing zero bias. This unusual $B$ dependence, which is remarkably independent of the charge state of the DQD, might be related to the hybrid nanowire/Al leads used in this experiment, which have shown zero-energy crossings in $B$ in the past [S27]. Notice that, consistently with our interpretation of the (1,0) sector as a doublet ground state, the peaks at its boundaries split apart due to Zeeman splitting.

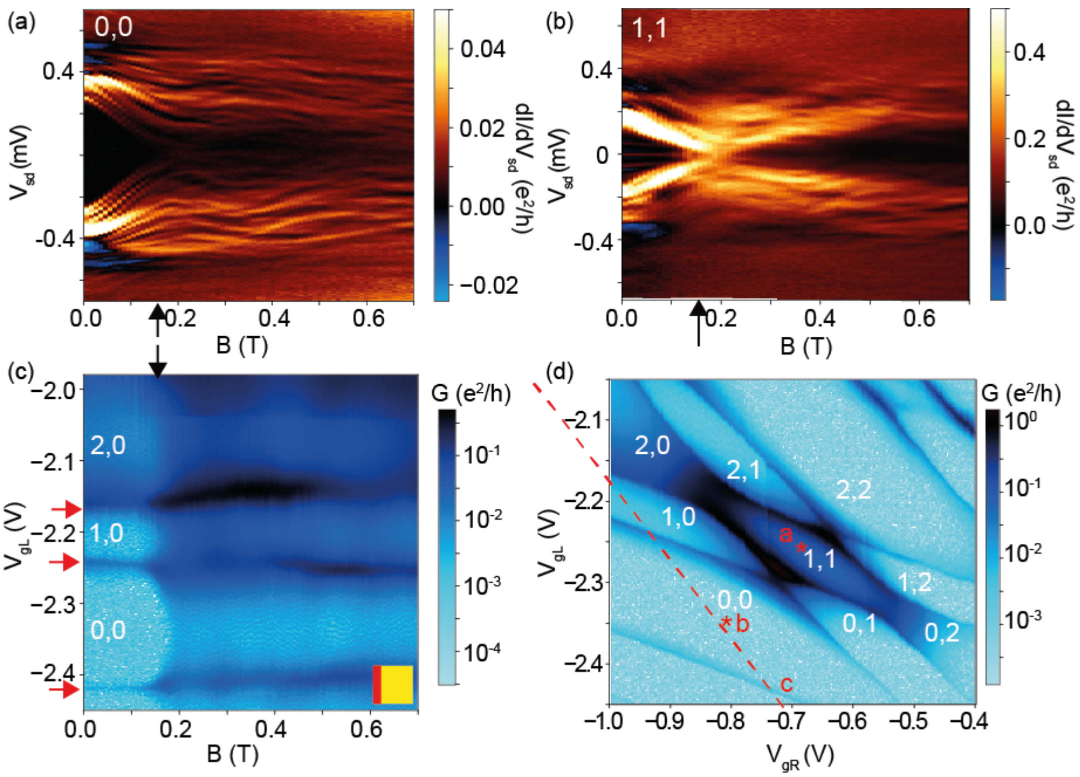


FIG. S4. (a,b) Magnetic field evolution of subgap features in the center of the (a) (0,0) and (b) (1,1) sectors. (c) $B$ dependence of the linear conductance through sectors (0,0),(1,0) and (2,0). In panels (a-c), vertical black arrows point to $B = 0.16$ T, which is the field at which subgap states cross zero bias. (d) Same as Fig. 2 of the main text, shown here to indicate the gate position of maps (a,b) (asterisks) and (c) (line-cut through dashed line).

## VI. (-1,1) AND (1,3) CHARGE SECTORS

Here we complement the supercurrent and subgap states data presented in the main article and above by showing $I_c$ and subgap states gate-dependence in other DQD shells. The stability diagrams of these sectors are depicted in Figs. S5a,d, which correspond to the same charge sectors indicated in Fig. S3a, but at a slightly different gate configuration. Interestingly, the diagram in Fig. S5a has a similar conductance pattern as the diagram presented in Fig. 1e of the main article -aside from the gate jumps-, whereas the diagram in in Fig. S5b has a noticeably different pattern, with a significantly smaller conductance. The $I_c$ line-cuts in Figs. S5b,e show that $I_c$ is also strongly reduced in charge sector (-1,1). These observations lead us to believe that the tunnel coupling in the latter is smaller than the one in the diagram of Fig. 1e or Fig. S5a, probably due to cross-tuning of $\Gamma_L$ by decreasing $V_{gL}$. In spite of these apparent differences, the critical current in these three diagrams behaves the same way as described in the main text; namely, an odd total occupation results in a doublet ground state. The same holds for YSR subgap states, an example of which is shown for each case in Figs. S5c,f.

## VII. SPECTROSCOPY OF THE CONVOLUTED GAP AND TEMPERATURE DEPENDENCE

In the regime of relatively strong coupling needed to observe supercurrent which was depicted in the main text, differential conductance measurements of the gap (e.g. Fig. S3) displayed a myriad of peaked sub-gap features. This peaked subgap conductance was observable when the backgate voltage was set at a positive value of 10.4 V.

In this section, we show that when there is a large negative voltage applied on the backgate ($V_{bg} = -15$ V) the gap becomes hard.

Fig. S6a shows the *honeycomb*-shaped double dot diagram in this opaque regime, obtained with the gates set at $V_{g2} = 2.25$ V, $V_{g3} = -6.5$ V, $V_{g5} = -6.5$ V, and $V_{bg} = -15$ V. Coincidentally, the shell-filling pattern has been lost. The absence of a significant level-spacing in this new gate configuration is also seen in a the line-cut shown in panel (b). Coulomb diamonds displayed in this panel show many excited levels closely spaced, being probed either in

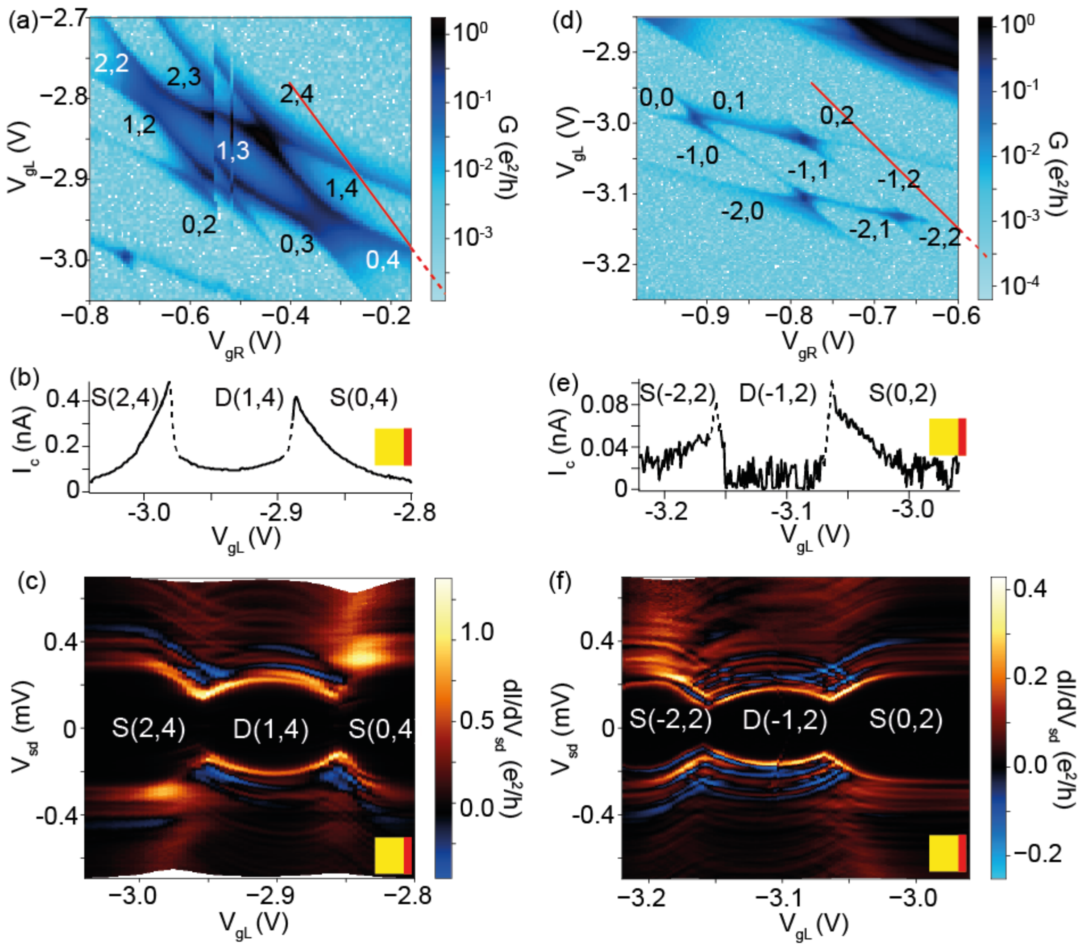


FIG. S5. (a,d) Zoom on the honeycomb stability diagrams around charge sectors (1,3) and (-1,1) indicated in Fig. S3a. Charges in each dot with respect to the charge numbers in the stability diagram depicted in the main article are indicated here as reference. In both cases, $V_{g1} = -9.2$ V, $V_{g3} = -9.0$ V, $V_{g5} = -0.36$ V. However, the backgate voltage was set differently; (a) $V_{bg} = 10.7$ V and (d) $V_{bg} = 11.0$ V. These gates were set so that each diagram corresponds to the low-coupling regime, and at the same time to push the plunger gates field away from the unstable region at $V_{gL} \approx -0.4$ V in Fig. S3a. The unstable region depended weakly on other gates as well, and still shows in panel (a). (b,e) Line-cuts of fitted $I_c$ through the red lines in panels (a) and (b). The ground state, as revealed by $I_c$ and subgap states gate dependence, is indicated in each sector of the plots. (c,f) Differential conductance maps taken through the red lines in panels (a) and (b), showing YSR subgap states with apparent replicas.

sequential tunneling or in cotunneling transport by the continuum singularities. The absence of even-odd alternation in this measurement indicates the multi-level regime of the dots in this new gate setting.

The superconducting gap splits the Coulomb diamonds by half in this map, and its hardness is evidenced by the absence of features at $\Delta$ at the charge degeneracy points, which would otherwise be an indication of a finite density of states at zero energy [S28]. Fig. S6c shows an $I - V_{sd}$ curve which represents the convolution of the superconducting gaps of the two leads, taken at $V_{g1} = 2.52$ V, near the middle of the rightmost Coulomb diamond of panel (b) (at the vertical dotted line), when $\Gamma_0 \ll U$, in the cotunneling regime. The voltages at which the current jumps from zero to a finite value allow us to accurately measure $2\Delta = 0.53$ mV. From Fig. S6d, which shows the temperature evolution of the convoluted gaps, we extract a critical temperature $T_c = 2.2$ K, and a ratio $2\Delta/T_c = 2.8$.

A large negative voltage can have two effects which might separately explain the observation of a hard gap. Firstly, strong depletion decreases the tunnel couplings to the leads, as evidenced by the sharp co-tunneling and sequential tunneling lines in Fig. S6b. The low coupling to the leads pushes YSR states out of the gap, which is consistent with a lack of crossings at the degeneracy points of Fig. S6b. Secondly, a negative backgate voltage may increase confinement in the nanowire sections below the Al leads, which would push away Andreev bound states in these sections. Clearing the gap from YSR or Andreev bound states clearly leads to a harder gap.

Finally, in Fig. S6e we show a measurement of the magnetic field dependence of the convoluted gaps, with $B$ aligned

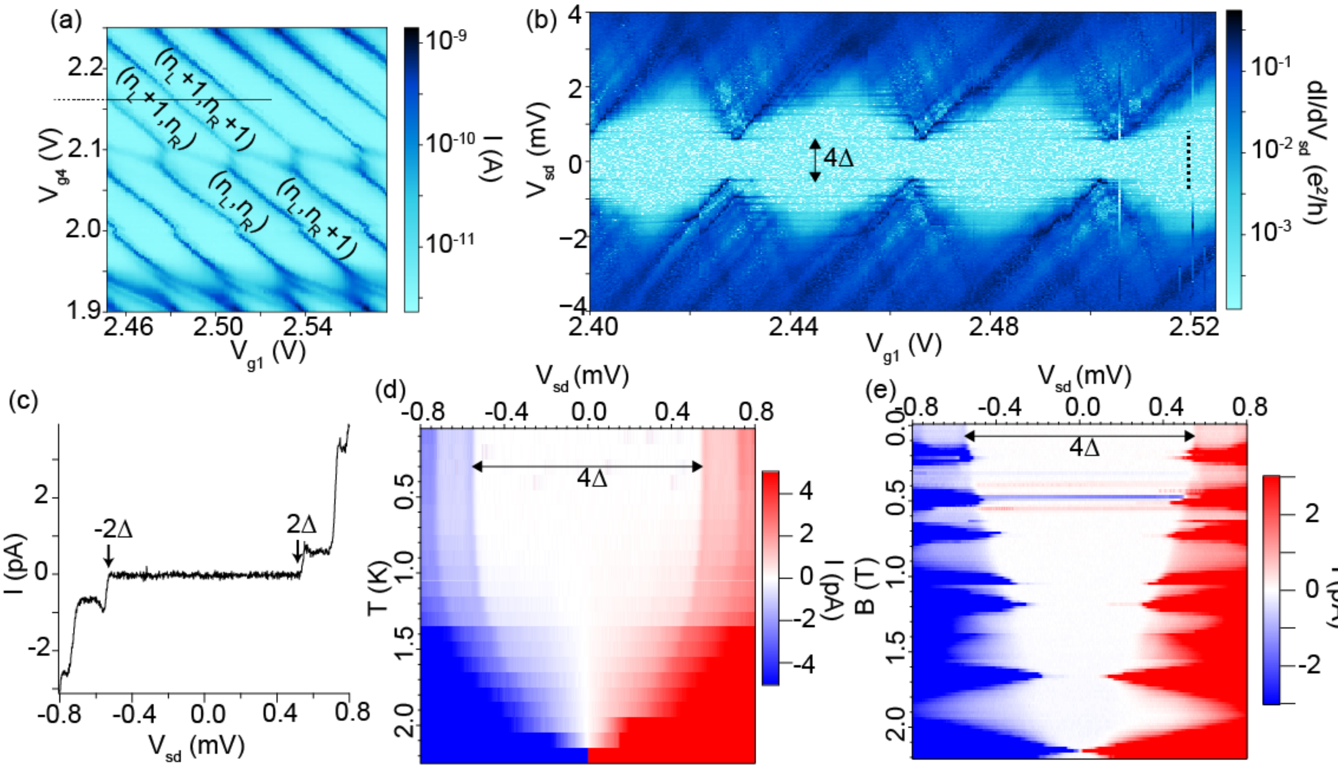


FIG. S6. (a) Double dot stability diagram measured with the bias voltage set at $V_{sd} = 0.54$ mV $\approx 2\Delta$, taken at $T = 25$ mK and at negative backgate voltage (see text for details). (b) Coulomb diamonds map taken through the black line in panel a. Two symmetric cotunneling features coming from the BCS peaks split the diamonds in two by a forbidden energy band of $4\Delta$. (c) I-V curve taken at $V_{g1} = 2.52$ V. This curve represents a convolution of the superconducting gap induced by one of the leads while probing the gap induced by the other lead. When the two BCS singularities of the gaps enter the bias window at $V_{sd} = 2\Delta$, a shoot-up of the current occurs. (d) Temperature evolution of the convoluted superconducting gaps.The colormap illustrates the temperature dependence of the I-V curve in panel (a). From this plot, we extract $T_c = 2.2$ K. (e) Magnetic field dependence of the convoluted gaps. The scale was saturated at both ends to emphasize the region of zero current.

to the long axis of the nanowire. In this opaque regime, the gap has a significantly cleaner $B$-evolution compared to the measurements with YSR states and their replicas in the more transparent regime of Figs. S4a,b. Notice that the gap remains hard over a large magnetic field range (aside from spurious charge instabilities at $B = 0.4 - 0.6$ T), as evidenced by zero current (white color). Above the gap, cotunneling lines due to excited states in the dots split in field and enter and leave the bias window as $B$ is stepped.

Backgate tuning of the number of subgap states has also been reported before in similar wires as used here, in an experiment on which the nanowire below a mesoscopic Al lead was turned into a topological superconductor by applying a magnetic field parallel to the long axis of the wire (see Supplemetary information of Ref. [S27]). In our case, it is not possible to decouple the density of states of the two hybrid wire/Al mesoscopic leads from dot-related YSR states, and thus we are not able to verify if the crossing of subgap states observed in Figs. S4a,b, which is independent of the charge in the dots, is related to hybrid wire/Al properties in one or both leads.

## VIII. THEORETICAL MODELS FOR SUPERCURRENT

We describe the full S-DQD-S system using a general two-orbital Anderson model coupled to two BCS leads,

$$H = H_D + H_{BCS} + H_T \tag{S3}$$

$$H_D = \sum_{\sigma,i=L,R} \frac{U_i}{2}(\bar{n}_{i\sigma} - n_i)^2 + \sum_{\sigma,\sigma'} U_{LR}(\bar{n}_{L\sigma} - n_L)(\bar{n}_{R\sigma'} - n_R) + t_d \sum_{\sigma} \left( d^\dagger_{L\sigma} d_{R\sigma} + d^\dagger_{R\sigma} d_{L\sigma} \right) \tag{S4}$$

$$H_{BCS} = \sum_{k,\sigma,i=L,R} \xi_i c^\dagger_{ik\sigma} c_{ik\sigma} + \sum_{k,i=L,R} \left( \Delta_i c^\dagger_{ik\uparrow} c^\dagger_{i-k\downarrow} + \Delta^*_i c_{i-k\downarrow} c_{ik\uparrow} \right) \tag{S5}$$

$$H_T = \sum_{k,\sigma,i=L,R} t_i \left( c^\dagger_{ik\sigma} d_{i\sigma} + d^\dagger_{i\sigma} c_{ik\sigma} \right) \tag{S6}$$

Here $\bar{n}_{i\sigma}$ denotes the electron occupation operator for dot $i = L, R$ with spin $\sigma =\uparrow,\downarrow$ while local gate voltages are used to tune the individual average dot occupations, $n_i$. For this serial double dot all tunnel couplings can be chosen real, as any spin-independent phase can be gauged onto the phase difference between the two superconducting order parameters, $\phi = \phi_L - \phi_R$. In this paper we consider the regime $|\Delta| = |\Delta_L| = |\Delta_R|$, $|\Delta| \ll U_i$ and $\Gamma_R, \Gamma_L \ll U_L, U_R$ with $\Gamma_i = \pi\nu_F |t_i|^2$ where $\nu_F$ is the assumed constant density of states in the superconducting leads. In this regime the dominant correlation between superconductors and dots is Yu-Shiba-Rusinov screening of spin-full states [S3]. In this paper we will only consider weak YSR correlations such that the stability diagram maintains its honeycomb pattern. [S17].

Using this Hamiltonian, we now calculate the supercurrent within 4$^{\text{th}}$ order perturbation in $H_T$ and by direct diagonalization within a zero-bandwidth approximation. For weak coupling, $\Gamma_i \ll |\Delta|, U_i$, this confirms the sinusoidal current-phase relation, $I = I_c \sin(\phi)$, and the critical current, $I_c$, is calculated and compared to that obtained by fitting the data to the RCSJ model, as discussed in the main text.

### A. Perturbation theory

The leading order contribution to Cooper pair transport across the junction is 4$^{\text{th}}$ order in $H_T$ [S29, S30], leading to the correct supercurrent for $\Gamma_R, \Gamma_L \ll U_i, |\Delta|$. This calculation does not include any dot renormalization from coupling them to superconducting leads and therefore does not include YSR correlations. The current running into the right lead is given by

$$I = i\frac{e}{\hbar} \sum_{\sigma} \langle [H, \bar{n}_{R\sigma}] \rangle = \frac{2e}{\hbar} \operatorname{Im} \sum_{\sigma} \langle H_{TR\sigma} \rangle, \tag{S7}$$

where we use the shorthand $H_{Ti\sigma} = t_i \sum_k c^\dagger_{ik\sigma} d_{i\sigma}$. Expanding the time evolution operator to lowest non-vanishing order yields,

$$I \approx -\frac{2e}{\hbar}\frac{1}{3!} \operatorname{Im} \frac{1}{\beta} \int_0^\beta \mathrm{d}\tau_1\, \mathrm{d}\tau_2\, \mathrm{d}\tau_3\, \mathrm{d}\tau_4 \sum_{\sigma} \Big\langle \mathrm{T}_\tau \left( H_T(\tau_1) H_T(\tau_2) H_T(\tau_3) H_{TR\sigma}(\tau_4) \right) \Big\rangle_0, \tag{S8}$$

where $\langle ... \rangle_0$ is the statistical average disregarding $H_T$, such that dots and leads are decoupled. In order for this to be non-zero, two electrons with opposite spin must be removed from one lead and added to the other. With 3 ways to order leads and 4 ways to order spin we obtain

$$I = -\frac{4e}{\hbar} \operatorname{Im} \frac{1}{\beta} \int_0^\beta \mathrm{d}\tau_1\, \mathrm{d}\tau_2\, \mathrm{d}\tau_3\, \mathrm{d}\tau_4 \Big\langle \mathrm{T}_\tau \left( H^\dagger_{TL\uparrow}(\tau_1) H^\dagger_{TL\downarrow}(\tau_2) H_{TR\downarrow}(\tau_3) H_{TR\uparrow}(\tau_4) \right) \Big\rangle_0 \tag{S9}$$

$$= -\frac{4e}{\hbar} t_L^2 t_R^2 \operatorname{Im} \frac{1}{\beta} \int_0^\beta \mathrm{d}\tau_1\, \mathrm{d}\tau_2\, \mathrm{d}\tau_3\, \mathrm{d}\tau_4 \mathcal{F}^*_L(\tau_1 - \tau_2) \mathcal{F}_R(\tau_3 - \tau_4) \mathcal{B}(\tau_1, \tau_2, \tau_3, \tau_4), \tag{S10}$$

where $\mathcal{F}$ is the momentum-summed anomalous Green function for the leads,

$$\mathcal{F}_i(\tau) = -\sum_p \Big\langle \mathrm{T}_\tau \left( c^\dagger_{i-p\downarrow}(\tau) c^\dagger_{ip\uparrow}(0) \right) \Big\rangle_0 = -\pi\nu_0 \frac{\Delta^*}{\beta} \sum_n \frac{e^{-i\omega_n \tau}}{\sqrt{\omega_n^2 + |\Delta|^2}}, \tag{S11}$$

and where $\mathcal{B}$ encodes all contributions from the double dot as

$$\mathcal{B}(\tau_1,\tau_2,\tau_3,\tau_4) = \left\langle \, \mathrm{T}_\tau \left( d_{L\uparrow}(\tau_1) d_{L\downarrow}(\tau_2) d^\dagger_{R\downarrow}(\tau_3) d^\dagger_{R\uparrow}(\tau_4) \right) \right\rangle_0 . \tag{S12}$$

In Eq.(S10) the phase dependence resides on $\Delta$, and taking the imaginary part one readily arrives at $I = I_c \sin(\phi)$, with

$$I_c = -\frac{4e}{\hbar} |\Delta|^2 \, \Gamma_R \Gamma_L \frac{1}{\beta} \int_0^\beta \mathrm{d}\tau_1 \, \mathrm{d}\tau_2 \, \mathrm{d}\tau_3 \, \mathrm{d}\tau_4 f^*(\tau_1-\tau_2) f(\tau_3-\tau_4) B(\tau_1,\tau_2,\tau_3,\tau_4), \tag{S13}$$

where $f(\tau) = \sum_n \frac{e^{-i\omega_n \tau}}{\sqrt{\omega_n^2 + |\Delta|^2}}$ . In order to simplify $\mathcal{B}$ for a serial double dot, we set $T=0$ such that we always have a definite DQD groundstate, $|g\rangle$, which depends on parameters and gate voltages. Since the system is spin-rotational invariant, a spin-degenerate ground state may be replaced by one specific spin projection, and in general Eq. (S12) therefore reduces to

$$\mathcal{B}(\tau_1,\tau_2,\tau_3,\tau_4) = \langle g | \, \mathrm{T}_\tau \left( d_{L\uparrow}(\tau_1) d_{L\downarrow}(\tau_2) d^\dagger_{R\downarrow}(\tau_3) d^\dagger_{R\uparrow}(\tau_4) \right) |g\rangle \, . \tag{S14}$$

This expression yields 24 different time orderings, which we consider one by one using the general object

$$\mathcal{B}_g = \langle g | \, d_a(\tau_a) d_b(\tau_b) d_c(\tau_c) d_d(\tau_d) \, |g\rangle \, , \tag{S15}$$

where the labels $a$, $b$, $c$ and $d$ can be any of the spin, lead and dagger sub- or superscripts above. First we expand $\mathcal{B}_g$ in the eigenstates of the uncoupled ($t_d = 0$) quantum dots, denoted by $|n_{1\uparrow}, n_{1\downarrow}, n_{2\uparrow}, n_{2\downarrow}\rangle$. In this basis the $d_{i\sigma}$ operators can be represented as off-diagonal matrices containing only $\pm 1$ denoted by $M_{i\sigma}$ for $d_{i\sigma}$. We then reinstate $t_d$ and diagonalize the dot subspace with a unitary transformation $U$ resulting in $U M_{i\sigma} U^\dagger = \bar{M}_{i\sigma}$ as the new off-diagonal matrices connecting dot subspaces of different electron number. For each choice of parameters the matrix $U$ is obtained numerically. Following this procedure, our generic $\mathcal{B}_g$ can be written as

$$\mathcal{B}_g = \sum_{n,m,l} (\bar{M}_a)_{gn} (\bar{M}_b)_{nm} (\bar{M}_c)_{ml} (\bar{M}_d)_{lg} e^{-\epsilon_n(\tau_a - \tau_b)} e^{-\epsilon_m(\tau_b-\tau_c)} e^{-\epsilon_l(\tau_c-\tau_d)}, \tag{S16}$$

where $\epsilon_l, \epsilon_m$, and $\epsilon_n$ are the excitation energies in the diagonal basis. Reinserting this generic form into Eq.(S13) we must for all cases match $\{\tau_a,\tau_b,\tau_c,\tau_d\}$ with $\{\tau_1,\tau_2,\tau_3,\tau_4\}$. Using the restriction $f(\tau) = f(-\tau) = f^*(\tau)$, only three different cases appear:

$$q_i(n,m,l) = \frac{1}{\beta}\int_0^\beta \mathrm{d}\tau_a \int_0^{\tau_a} \mathrm{d}\tau_b \int_0^{\tau_b} \mathrm{d}\tau_c \int_0^{\tau_c} \mathrm{d}\tau_d e^{-\epsilon_n(\tau_a-\tau_b)} e^{-\epsilon_m(\tau_b-\tau_c)} e^{-\epsilon_l(\tau_c-\tau_d)} \begin{cases} f(\tau_a-\tau_b) f(\tau_c-\tau_d), & i=1 \\ f(\tau_a-\tau_d) f(\tau_c-\tau_b), & i=2 \\ f(\tau_a-\tau_c) f(\tau_b-\tau_d), & i=3 \end{cases} \tag{S17}$$

these integrals can be evaluated for $T=0$ and after analytical continuation we arrive at

$$q_i(i,j,k) = \frac{1}{\pi^2 \Delta^3} Q_i(i,j,k), \tag{S18}$$

given in terms of the scale-free and strictly positive quantity

$$Q_i(n,m,l) = \int_1^\infty \int_1^\infty \frac{\mathrm{d}\omega_1 \, \mathrm{d}\omega_2}{\sqrt{\omega_1^2-1}\sqrt{\omega_2^2-1}} \begin{cases} \dfrac{1}{(\epsilon_n/\Delta+\omega_1)(\epsilon_l/\Delta+\omega_2)(\epsilon_m/\Delta)}, & i=1 \\ \dfrac{1}{(\epsilon_n/\Delta+\omega_1)(\epsilon_l/\Delta+\omega_1)(\epsilon_m/\Delta+\omega_1+\omega_2)}, & i=2 \\ \dfrac{1}{(\epsilon_n/\Delta+\omega_1)(\epsilon_l/\Delta+\omega_2)(\epsilon_m/\Delta+\omega_1+\omega_2)}, & i=3 \end{cases} \tag{S19}$$

The time ordering determines in what electronic sequence a Cooper pair is transferred through the system, and the three different contributions are referred to by the index $i = 1,2,3$. Diagrammatically the three orderings, along with the scale of their contribution to $I_c$ is shown in Fig. S7. $Q_1$ corresponds to the case of a full Cooper pair being added(removed) to the dots and then removed(added) such that $\epsilon_m$ is always two electrons away from the groundstate. This forces $\epsilon_m \geq U$ such that these processes in total scale as $I_c \propto \Gamma_R\Gamma_L/U$. $Q_3$ corresponds to the processes, where single quasiparticles tunnel through the dots one at a time, associated with a cost of $\Delta$, for temporarily splitting

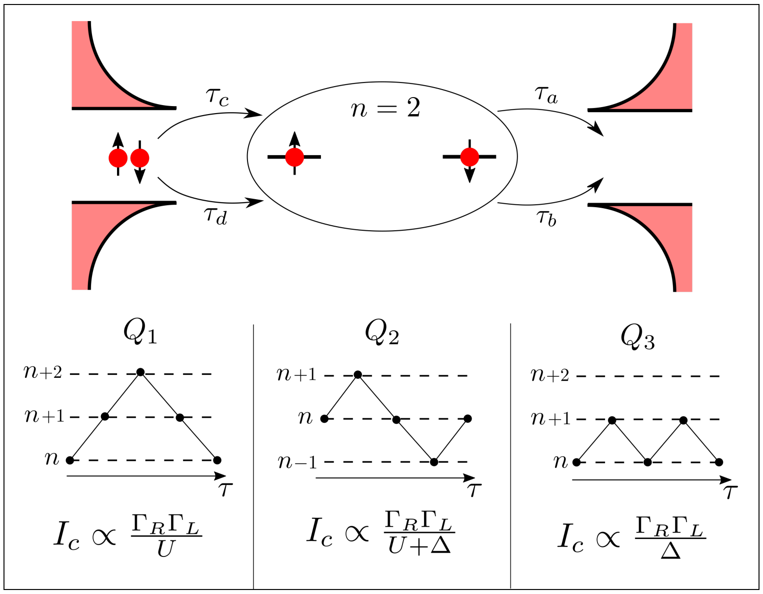


FIG. S7. Illustrating the four processes nessersary to transport a Cooper pair across the serial DQD. Considering all possible orderings, only three different processes, $Q_1, Q_2$ and $Q_3$, contribute at zero temperature. For each such process a diagram showing its related change in total dot electron number, $n$, is shown. As indicated, each process contributes to $I_c$ with a different energy denominator.

the Cooper pair. These processes therefore scale as $I_c \propto \Gamma_R\Gamma_L/\Delta$ instead. Lastly, the $Q_2$ is associated with both splitting the Cooper pair and changing the groundstate by two electrons and is therefore associated with the scale $I_c \propto \Gamma_L\Gamma_R/(\Delta + U)$.

To map out the full charge diagram one needs to obtain $I_c$ for all electron occupations of the serial DQD. For a given ground state we find all non-zero orderings in Eq. (S14), which provide both the overall sign of the contributions and the corresponding integral $Q_i(n, m, l)$. For each ordering we then sum over all paths through the system and

finally add up the contributions from all orderings. This yields

$$I_c(n=0) = \frac{4e\Gamma_L\Gamma_R}{\pi^2\hbar\Delta}\Bigg[\sum_{\sigma}\sum_{i,k\in n=1}(\bar{M}_{L\sigma})_{gi}(\bar{M}_{R\sigma})_{ig}(\bar{M}_{L\bar{\sigma}})_{gk}(\bar{M}_{R\bar{\sigma}})_{kg}Q_3(i,g,k) \tag{S20}$$

$$+\sum_{\sigma,\sigma'}\sigma\sigma'\sum_{i,k\in n=1}\sum_{j\in n=2}(\bar{M}_{L\sigma})_{gi}(\bar{M}_{L\bar{\sigma}})_{ij}(\bar{M}_{R\bar{\sigma}'})_{jk}(\bar{M}_{R\sigma'})_{kg}Q_1(i,j,k)\Bigg],$$

$$I_c(n=1,\uparrow) = \frac{4e\Gamma_L\Gamma_R}{\pi^2\hbar\Delta}\Bigg[-\sum_{j\in n=1}(\bar{M}_{R\uparrow})_{g0}(\bar{M}_{L\downarrow})_{0i}(\bar{M}_{R\downarrow})_{i0}(\bar{M}_{L\uparrow})_{0g}Q_3(0,j,0) \tag{S21}$$

$$-\sum_{i,k\in n=2}\sum_{j\in n=1}(\bar{M}_{L\downarrow})_{gi}(\bar{M}_{R\uparrow})_{ij}(\bar{M}_{L\uparrow})_{jk}(\bar{M}_{R\downarrow})_{kg}Q_3(i,j,k)$$

$$+\sum_{i,k\in n=2}\sum_{j\in n=1}(\bar{M}_{L\uparrow})_{gi}(\bar{M}_{R\uparrow})_{ij}(\bar{M}_{L\downarrow})_{jk}(\bar{M}_{R\downarrow})_{kg}Q_3(i,j,k)$$

$$+\sum_{i,k\in n=2}\sum_{j\in n=1}(\bar{M}_{L\downarrow})_{gi}(\bar{M}_{R\downarrow})_{ij}(\bar{M}_{L\uparrow})_{jk}(\bar{M}_{R\uparrow})_{kg}Q_3(i,j,k)$$

$$+\sum_{\sigma}\sigma\sum_{i\in n=2}\sum_{j\in n=1}(\bar{M}_{L\downarrow})_{gi}(\bar{M}_{R\sigma})_{ij}(\bar{M}_{R\bar{\sigma}})_{j0}(\bar{M}_{L\uparrow})_{0g}Q_2(i,j,0)$$

$$+\sum_{\sigma}\sigma\sum_{j\in n=1}\sum_{k\in n=2}(\bar{M}_{R\uparrow})_{g0}(\bar{M}_{L\bar{\sigma}})_{0j}(\bar{M}_{L\sigma})_{jk}(\bar{M}_{R\downarrow})_{kg}Q_2(0,j,k)$$

$$+\sum_{\sigma\sigma'}\sigma\sigma'\sum_{i,k\in n=2}\sum_{k\in n=3}(\bar{M}_{L\sigma})_{gi}(\bar{M}_{L\bar{\sigma}})_{ij}(\bar{M}_{R\bar{\sigma}'})_{jk}(\bar{M}_{R\sigma})_{kg}Q_1(i,j,k)\Bigg],$$

and

$$I_c(n=2) = \frac{4e\Gamma_L\Gamma_R}{\pi^2\hbar\Delta}\sum_{\sigma\sigma'}\sigma\sigma'\Bigg[+\sum_{i,k\in n=1}\sum_{j\in n=2}(\bar{M}_{R\sigma})_{gi}(\bar{M}_{L\sigma'})_{ij}(\bar{M}_{R\bar{\sigma}})_{jk}(\bar{M}_{L\bar{\sigma}'})_{kg}Q_3(i,j,k) \tag{S22}$$

$$+\sum_{i,k\in n=3}\sum_{j\in n=2}(\bar{M}_{L\sigma})_{gi}(\bar{M}_{R\sigma'})_{ij}(\bar{M}_{L\bar{\sigma}})_{jk}(\bar{M}_{R\bar{\sigma}'})_{kg}Q_3(i,j,k)$$

$$+\sum_{i\in n=1}\sum_{j\in n=2}\sum_{k\in n=3}(\bar{M}_{R\sigma})_{gi}(\bar{M}_{L\bar{\sigma}'})_{ij}(\bar{M}_{L\sigma'})_{jk}(\bar{M}_{R\bar{\sigma}})_{kg}Q_2(i,j,k)$$

$$+\sum_{i\in n=3}\sum_{j\in n=2}\sum_{k\in n=1}(\bar{M}_{L\sigma})_{gi}(\bar{M}_{R\bar{\sigma}'})_{ij}(\bar{M}_{R\sigma'})_{jk}(\bar{M}_{L\bar{\sigma}})_{kg}Q_2(i,j,k)$$

$$+\sum_{i,k\in n=1}(\bar{M}_{R\sigma})_{gi}(\bar{M}_{R\bar{\sigma}})_{i0}(\bar{M}_{L\bar{\sigma}'})_{0k}(\bar{M}_{L\sigma'})_{kg}Q_1(i,0,k)$$

$$+\sum_{i,k\in n=3}(\bar{M}_{L\sigma})_{gi}(\bar{M}_{L\bar{\sigma}})_{i4}(\bar{M}_{R\bar{\sigma}'})_{4k}(\bar{M}_{R\sigma'})_{kg}Q_1(i,4,k)\Bigg].$$

Utilizing particle-hole symmetry, one finds correspondingly that $I_c(n=3)$ and $I_c(n=4)$ may be obtained using the relations $I_c(n_L, n_R) = I_c(2-n_L, 2-n_R)$ where $n_{L/R}$ correspond to gate-voltages which are now tuned to give either a three, or a four-electron groundstate. Notice that these gate-voltages enter the expressions above through the $\bar{M}$ matrices. Using these expressions, we can calculate $I_c$ for the entire stability diagram for a serial double dot.

### B. Zero-Bandwidth approximation

As was recently demonstrated in Ref. [S17], a zero-bandwidth (ZBW) approximation for the BCS leads reproduces the correlations leading to YSR bound states very well and compares even quantitatively, after a slight rescaling of

$\Gamma_0$, with results of a numerical renormalization group (NRG) calculation. Here we explore the possibility of utilizing this ZBW approximation to calculate the critical current $I_c$ and compare it to $4^{\text{th}}$ order perturbation theory. This approach provides a relatively easy way of assessing the effects of both finite temperature and finite (non-infinitesimal) $\Gamma_0$ on the $I_c$ profiles.

The basic principle of ZBW is to replace the superconducting leads by a single quasiparticle with energy $\pm|\Delta|$, equivalent to the following modification of the BCS Hamiltonian

$$H_{BCS} \approx H_{ZBW} = \sum_{i=L,R} \left( \Delta_i c_{i\uparrow}^\dagger c_{i\downarrow}^\dagger + \Delta_i^* c_{i\downarrow} c_{i\uparrow} \right). \tag{S23}$$

This reduces the Hilbert space of Eq. (S3) to $4^4 = 256$ states, which can be handled numerically by exact diagonalization. Calculating the free energy from the eigenenergies, $E_i$, of this ZBW Hamiltonian,

$$F(\phi) = -T \log \sum_i e^{-E_i(\phi)/T}, \tag{S24}$$

the supercurrent can be obtained as

$$I(\phi) = \frac{2e}{\hbar} \partial_\phi F(\phi), \tag{S25}$$

where $\phi = \phi_L - \phi_R$ denotes the phase difference. For small coupling, $\Gamma_0 \ll |\Delta|, U$ and zero temperature, this numerical procedure confirms the sinusoidal current-phase relation, $I = I_c \sin\phi$, obtained above within $4^{th}$ order perturbation (4PT) theory. Since only $|I_c|$ is measured in the experiment, we shall henceforth work with $I_c$ defined as

$$I_c = \max_\phi |I(\phi)|, \tag{S26}$$

which holds true regardless of whether the current-phase relation is sinusoidal or not. Next, we compare the results of ZBW with 4PT in the regime of $\Gamma_0 \ll |\Delta|, U$ and $T = 0$. By direct comparison (cf. Fig. S8, panels a and c), we find qualitatively the same behavior with ZBW and 4PT. In order to explore the limits of ZBW, we compare it to a reduced 4PT in which the integrals in Eq. (S18) are replaced by

$$Q_{i,Red}(n,m,l) = \begin{cases} \dfrac{1}{(\epsilon_n/\Delta+1)(\epsilon_l/\Delta+1)(\epsilon_m/\Delta)}, & i=1 \\ \dfrac{1}{(\epsilon_n/\Delta+1)(\epsilon_l/\Delta+1)(\epsilon_m/\Delta+2)}, & i=2 \\ \dfrac{1}{(\epsilon_n/\Delta+1)(\epsilon_l/\Delta+1)(\epsilon_m/\Delta+2)}, & i=3, \end{cases} \tag{S27}$$

which is similar to replacing the BCS density of states with peaks at $\pm|\Delta|$ like in the ZBW approach. Using this reduced 4PT, we obtain $I_c$ in exact agreement with $I_c$ from ZBW when using the scaling $\Gamma_{ZBW} = 2\Gamma_0/(\nu_F \Delta)$ and choosing $\Gamma_0$ small enough to effectively suppress any renormalization from the leads. This correspondence is shown in Fig. S8.

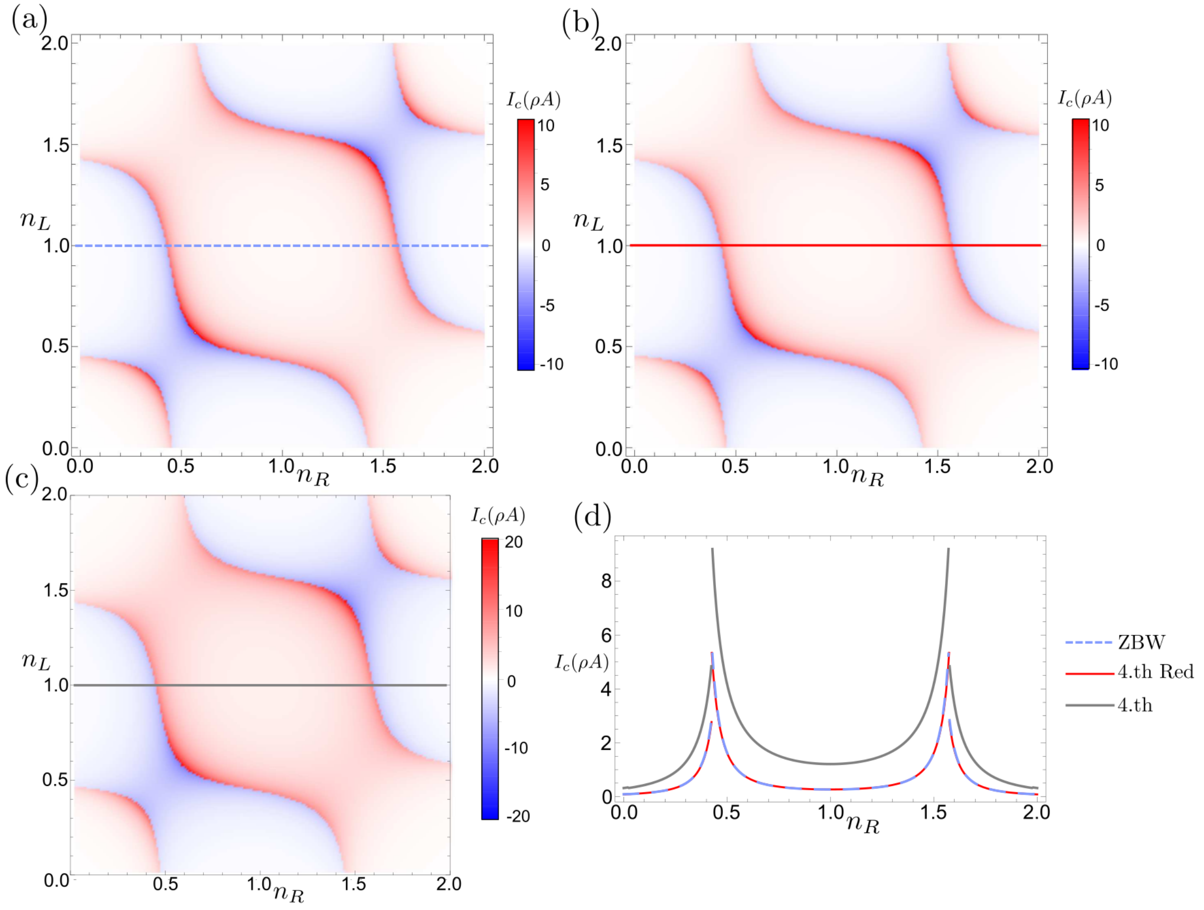


FIG. S8. (a), (b) and (c) are $I_c$ charge diagrams computed using respectively ZBW, reduced 4PT and full 4PT. The parameters used are $U_1 = U_2 = 4$ meV, $\Delta = 0.25$ meV, $t_d = 0.6$ meV, $U_{12} = 0$ meV, $\Gamma_L = \Gamma_R = 0.008$ meV, $T = 0$ meV. (d) shows three linecuts of $|I_c|$ through the stability diagrams corresponding to the respective lines in panels (a-c).

## IX. NUMERICAL RENORMALIZATION GROUP

Numerical renormalization group (NRG) is an iterative exact-diagonalisation technique based on a logarithmic discretization of the continuum of states in the (superconducting) leads [S31–S36]. The discretization is controlled by a parameter $\Lambda$ which determines the interval widths: $E_n \propto \Lambda^{-n}$, where $n$ is the interval index [S31]. This gives a good description of the low-energy energy scales, while the oscillatory artifacts resulting from a coarser discretization at higher energies can be to a large degree removed by averaging over several interleaved discretization grids [S37–S40] indexed by a twist parameter $z \in (0 : 1]$. It was observed that the results are greatly improved already by averaging over only two values of $z$ [S40, S41]. This makes it possible to perform calculation at very large values of the discretization parameter $\Lambda$, such as $\Lambda = 10$, which is necessary for handling demanding multi-channel problems with low symmetry [S41–S45] (in this work, the Hamiltonian only has SU(2) spin rotation invariance, and furthermore complex-number floating point arithmetics is required).

The BCS Hamiltonian in Eq. (S5) can be transformed by a unitary transformation $c_{Lk\sigma} \to f_{Lk\sigma} e^{i\phi_L/2}$, $c_{Rk\sigma} \to f_{Rk\sigma} e^{\phi_R/2}$ to a real form. We furthermore write $\phi_L = \phi/2$, $\phi_R = -\phi/2$. The phase dependence now only appears in the hopping terms:

$$H_T = \sum_{k\sigma} \left( t_L e^{i\phi/4} f_{Lk\sigma} d_{L\sigma} + t_R e^{-i\phi/4} f_{Rk\sigma} d_{R\sigma} \right) + \text{H.c.} \tag{S28}$$

The Josephson current is calculated at zero temperature through the energy derivative

$$J = \frac{2e}{\hbar} \frac{\partial E}{\partial \phi}. \tag{S29}$$

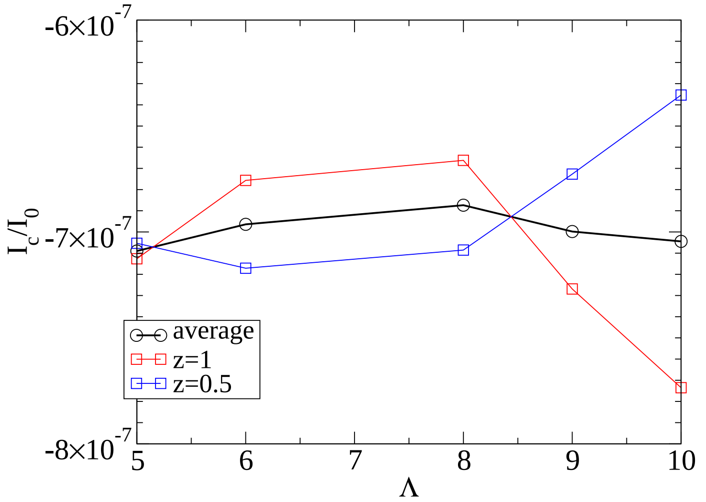


FIG. S9. The critical current $I_c$ in units of the transparent-junction limiting value of $I_0 = e\Delta/\hbar$. The fourth-order perturbation theory result is $I_c/I_0 = 7.02\times10^{-7}$. The parameters are $U = \infty$, $\epsilon = -2\Delta$, $\Delta = 0.0265D$, $\rho = 1/(2D)$, where $D$ is the bandwidth of the finite flat-band, and $\Gamma_L = \Gamma_R = 10^{-4}D$. All calculations are fully converged with respect to the NRG truncation (number of states retained in the calculation).

By Hellmann-Feynman theorem, $\partial E/\partial\phi = \langle\partial H/\partial\phi\rangle$, thus

$$\begin{aligned} J &= \frac{2e}{\hbar}\langle\hat{X}\rangle, \\ \hat{X} &= \frac{\partial H_T}{\partial\phi} \\ &= \frac{i}{4}\sum_{k\sigma}\left(t_L e^{i\phi/4} f_{Lk\sigma} d_{L\sigma} - t_R e^{-i\phi/4} f_{Rk\sigma} d_{R\sigma}\right) + \text{H.c.} \end{aligned} \tag{S30}$$

Operator $\hat{X}$ is local (in the NRG sense, i.e., it is defined on the initial cluster of the NRG calculation), thus its expectation value can be easily obtained. We have validated this approach for a single quantum dot problem by computing the critical current of a non-interacting resonant-level model at fixed gap $\Delta$ for a range of hybridization strengths $\Gamma_0$, equal for both leads, and comparing against exact expression in Eq. (8) of Ref. S46, finding an excellent agreement even at large $\Lambda$. As a further test we considered the $U = \infty$ limit of the Anderson model in the limit of low $\Gamma_0$, where simple expressions are available within the fourth-order perturbation theory [S47, S48]. Again we find good agreement. An NRG discretization parameter convergence study is shown in Fig. S9. The agreement between the perturbation theory result and the NRG results is quite satisfactory for all values of $\Lambda$ considered.

### A. Γ-dependence of the Josephson current

On the simplified case of a single quantum dot at $U = \infty$, we further investigated the domain of validity of the fourth-order perturbation theory, which is a good approximation to the true result at low $\Gamma$, but shows deviations at higher values of $\Gamma$ due to high-order processes (we note that the problem is actually non-perturbative in $\Gamma$, thus there is no power-series expansion around $\Gamma = 0$). In Fig. S10 we plot the critical current as a function of $\Gamma_0$ (single-dot hybridization per lead, $\Gamma_0 \equiv \Gamma_L = \Gamma_R$) at energy level $\epsilon = 0$, for $\Delta = 0.0265D$. We find that asymptotically the critical current indeed behaves quadratically, as expected, but the approach to this limit is rather slow. Even at $\Gamma_0/\Delta = 0.1$, the deviation between the (extrapolated) quadratic line and the actual NRG result is appreciable. This suggests that the fourth-order perturbation theory would significantly overestimate the actual Josephson current at this value. In the limit of small $\Gamma_0$, the Josephson current is sinusoidal to a very good approximation. It is thus maximal in absolute value at $\phi = \pi/2$. In this regime, it is hence sufficient to perform the calculation for a single

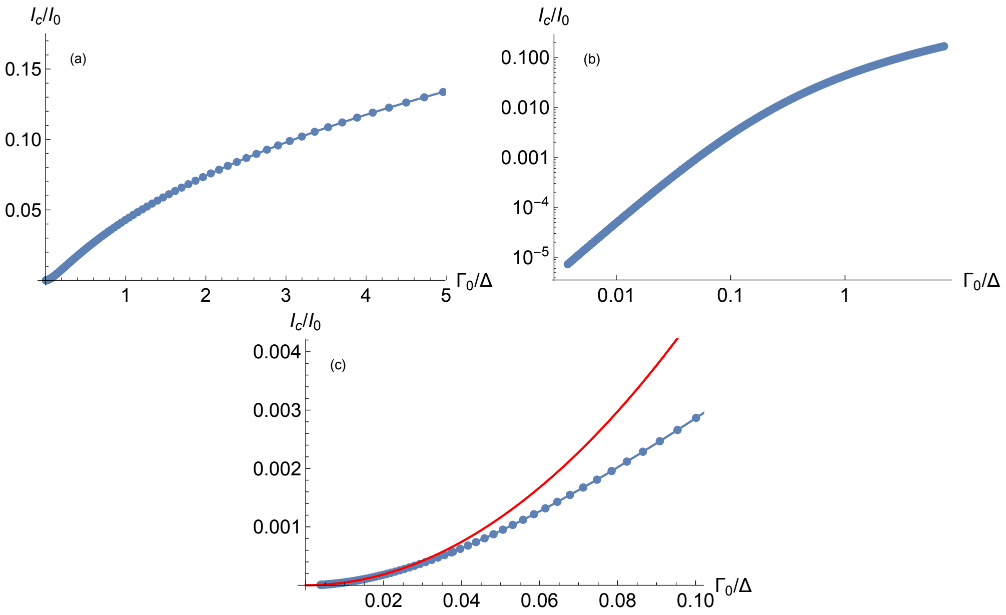


FIG. S10. Critical current for the single quantum dot problem at $U = \infty$, for $\epsilon = 0$ and $\Delta = 0.0265D$, as a function of the hybridisation strength per lead scaled by the BCS gap. (a) Linear plot. (b) Log-log plot. (c) Linear plot, close-up to low $\Gamma_0$, with a quadratic fit to low-$\Gamma_0$ results.

value of $\phi$. In general, however, higher harmonics in $\phi$ become important, thus one needs to perform a sweep over $\phi$ and the calculation becomes numerically significantly costlier. It turns out that for all the cases considered by NRG in this work, the system is indeed in the weak coupling regime and the maximum is always located essentially at $\pi/2$.

### B. NRG results for the S-DQD-S problem

Here we present the NRG calculations that support the fourth-order perturbation theory results in the main text of this work. Model parameters are $\Gamma_L = \Gamma_R = 0.01D$, $\Delta = 0.025D$, $U = 0.2D$, $t = 0.03D$. Here $D$ is the half-bandwidth of the conduction bands used in the NRG calculations. This choice of scaling corresponds to the wide-band limit where the bandwidth is the largest energy scale in the problem. We then used $D = 10\,\text{meV}$ to convert the parameters back to the energy units. In particular, $\Gamma_L = \Gamma_R = 0.1\,\text{meV}$. In Fig. S11 we show an overview diagram which delinates the singlet and doublet regimes of the system by representing in color the energy difference between the lowest singlet and lowest doublet states. The red line indicates the contour of zero difference (degeneracy of the sub-gap states, i.e., the quantum phase transition line), while the neighboring black lines indicate the contours of absolute value 0.1 (i.e. energy splitting $0.1\Delta$), so as to indicate the width of the transition region (here, in the weak-coupling limit, it is narrow). The Josephson current calculations have been performed along the cuts presented in the main text, see Figs. S12. In all cuts we used $\Gamma_L = \Gamma_R = 0.1$ meV close to the value $\Gamma_L = \Gamma_R = 0.08$ meV used to fit supercurrent by 4PT. In all cases we find good agreement between the methods.

Finally, in Fig. S13 we show the gate-voltage dependence of the sub-gap states along the $n_L = 1$ line. In addition to the lowest-lying singlet and doublet states that were discussed so far (and fully determine the Josephson current across the junction at $T = 0$), we find one additional singlet state, one doublet, and one triplet. Generally, we expect to find two singlet states within the gap because they correspond to two orthogonal combinations of elementary singlet states, $S_{\text{AFM}}$, which is the inter-impurity singlet state arising from the antiferromagnetic exchange coupling between the dots, and $S_{2\text{K}}$, which is a product state of two separate Kondo screened states. In the two-impurity Anderson model, the states $S_{\text{AFM}}$ and $S_{2\text{K}}$ mix: one combination is the singlet which becomes the ground state for $n_L = n_R = 1$, the other is an excited singlet state (which for other parameter values may merge with the continuum). In the two-impurity Kondo model, there may be a quantum phase transition between the two symmetrically different singlet states [S44]. For $\Gamma_0 = 0.1\,\text{meV}$, the singlet ground state at $n_L = n_R = 1$ is predominantly of the $S_{\text{AFM}}$ character, as evidenced by the expectation value of the spin-spin correlation, $\langle \mathbf{S}_L \cdot \mathbf{S}_R \rangle \approx -0.6$, close to the saturated value of $-3/4$. The doublet states correspond to the molecular-orbitals discussed in the main text. In our model with $U_L = U_R$, they become degenerate for $n_L = n_R = 1$, as seen here. Finally, the triplet state is the ferromagnetic-alignment counterpart of the

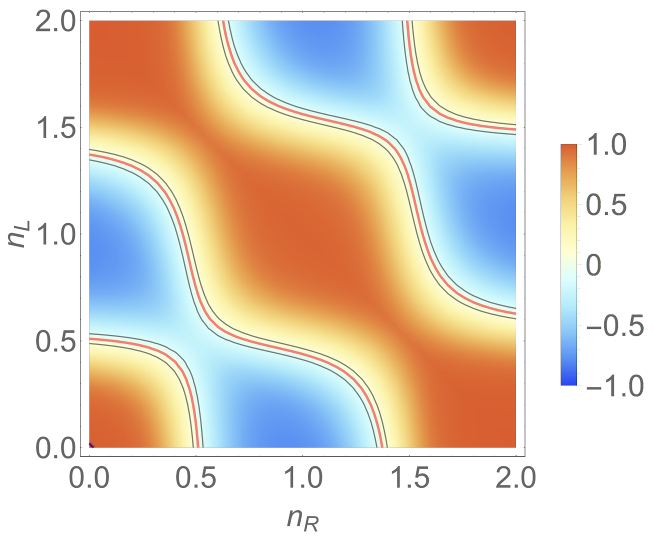


FIG. S11. Diagram presenting the energy difference between the sub-gap singlet and doublet states. The color scale is in units of the BCS gap $\Delta$, red corresponds to singlet ground-state, blue to a doublet ground-state.

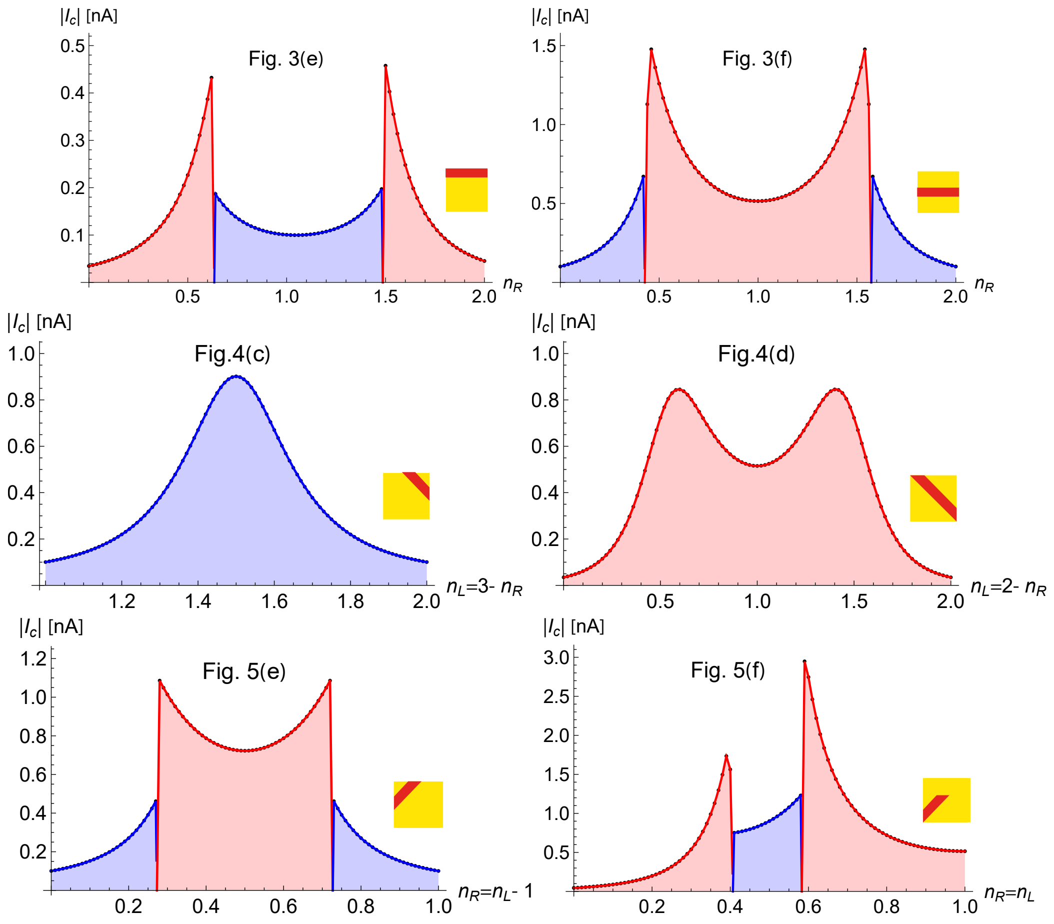


FIG. S12. Line-cuts of $|I_c|$ calculated by the numerical renormalization group (NRG) along the same trajectories as the fourth order perturbation-theory results in the main text. Red (blue) color indicates that $I_c$ is positive (negative). The plots are labeled by the Figure numbers from the main text for easier comparison.

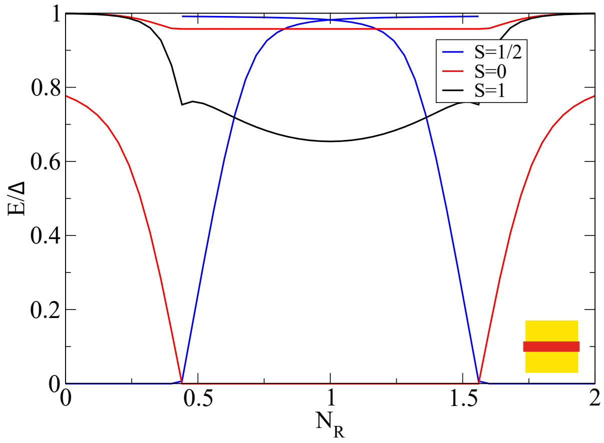


FIG. S13. Energies of the many-body eigenstates of the Hamiltonian below the edge of continuum excitations, i.e., the YSR sub-gap states. We show a cut along the $n_L = 1$ line.

antiferromagnet-alignment $S_{\mathrm{AFM}}$ singlet state. Such states have not been observed so far due to their low spectral weight [S17].

## X. $I_c$ CROSSINGS AT THE $0-\pi$ TRANSITION

At zero temperature, the $0-\pi$ transition is accompanied by an abrupt change in $I_c$, as predicted by 4PT, ZBW and NRG. At a finite temperature, however, the sharp ground state transition turns into a thermal mixture of nearly degenerate states, and the abrupt change in $I_c$ is disrupted by a sharp dip, which widens with increasing temperature. This is illustrated in Fig. S14, where $I_c$ is calculated within the ZBW approximation at temperature corresponding to that of the experiment. Fig. S14 shows four line cuts calculated using Eq. S26, all of which display sharp dips in the critical current at their respective $0-\pi$ transitions. Panels (f) show five current-phase relations corresponding to five different gate voltages near the transtion in panel (d). From left to right (increasing $n_R = n_L$ in panel (d)), a sinusoidal (0) relation develops through an intermediate non-sinusoidal ($0'$) relation to a $\pi$-periodic relation right at the minimum of the dip in $I_c$. A further increase in gate voltage takes the system through a non-sinusoidal ($\pi'$) relation and finally into the sinusoidal ($\pi$) relation in the right-most panel. Here we have used the labeling used in Refs. [S3, S49] dealing with the $0-\pi$ transition in a single-orbital Anderson model. We note that this evolution of current-phase relations across the $0-\pi$ transition is consistent with recent experiments on single-dot junctions in the underdamped regime, which have shown that $I_c$ does not go to zero at the $0-\pi$ transition [S50]. We attribute the fact that our experiment showed no such dips in $I_c$ in part to lack of resolution, since the peaks will be very narrow for $U \gg \Delta, \Gamma_0, T$, but also to inaccuracies in the fitting, which assumes a sinusoidal current-phase relation everywhere. This error has been discussed earlier in Ref. [S7].

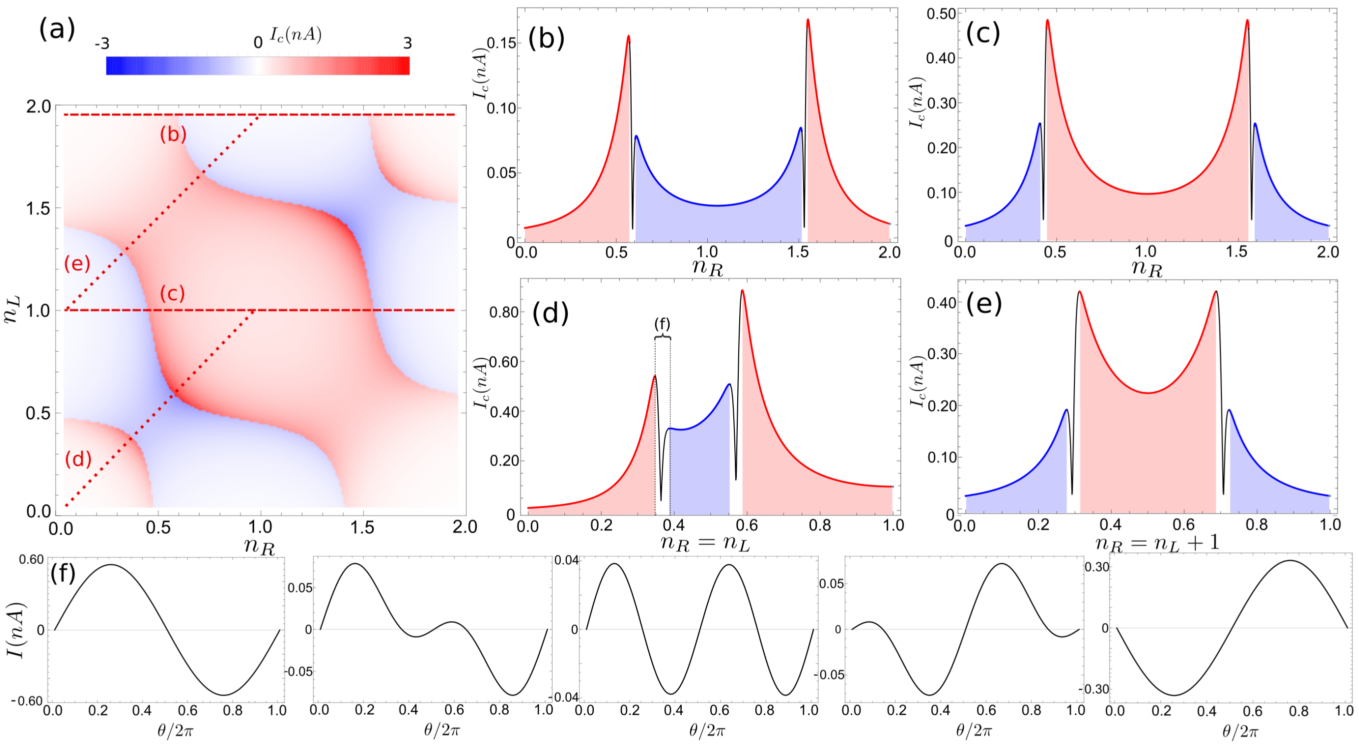

FIG. S14. (a) $I_c$ charge diagram calculated using 4PT and parameters from the main article. Blue lines show the corresponding linecuts (b-e). (b-e) $I_c = \max_\phi |I(\phi)|$ calculated using ZBW at finite temperature $T = 77.3$ mK and using parameters from the main article. The interval shown on (d) indicates the range of gate for which phase-current relations on (f) are provided. Panels (f) show the current-phase relations obtained at the corresponding gate (from left to right) $n_L = n_R = \langle 0.348, 0.363, 0.364, 0.365, 0.39\rangle$, calculated with ZBW using the same parameters as in (b-e) and the rescaling $\Gamma_{ZBW} = 2\Gamma_0/(\nu_F \Delta)$.


[S1] H. I. Jørgensen, K. Grove-Rasmussen, K.-Y. Wang, A. Blackburn, K. Flensberg, P. E. Lindelof, and D. Williams, Nat. Phys. **4**, 536 (2008).
[S2] J. A. Van Dam, Y. V. Nazarov, E. P. Bakkers, S. De Franceschi, and L. P. Kouwenhoven, Nature **442**, 667 (2006).
[S3] G. Kiršanskas, M. Goldstein, K. Flensberg, L. I. Glazman, and J. Paaske, Phys. Rev. B **92**, 235422 (2015).
[S4] A. Steinbach, P. Joyez, A. Cottet, D. Esteve, M. Devoret, M. Huber, and J. M. Martinis, Phys. Rev. Lett. **87**, 137003 (2001).
[S5] Y. M. Ivanchenko and L. A. Zil'berman, Soviet Physics Jetp **28**, 1272 (1969).
[S6] V. Ambegaokar and B. I. Halperin, Phys. Rev. Lett. **23**, 274 (1969).
[S7] H. I. Jørgensen, T. Novotný, K. Grove-Rasmussen, K. Flensberg, and P. E. Lindelof, Nano Lett. **7**, 2441 (2007).
[S8] A. Eichler, R. Deblock, M. Weiss, C. Karrasch, V. Meden, C. Schönenberger, and H. Bouchiat, Phys. Rev. B **79**, 2 (2009).
[S9] J. C. Estrada Saldaña, R. Žitko, J.-P. Cleuziou, E. J. H. Lee, V. Zannier, D. Ercolani, L. Sorba, R. Aguado, and S. De Franceschi, arXiv preprint arXiv:1801.01855 (2018).
[S10] P. Jarillo-Herrero, J. A. Van Dam, and L. P. Kouwenhoven, Nature **439**, 953 (2006).
[S11] In the fit, it is possible to keep $R_J$ constant because of the hard gap.
[S12] E. J. Lee, X. Jiang, M. Houzet, R. Aguado, C. M. Lieber, and S. De Franceschi, Nat. Nanotechnol. **9**, 79 (2014).
[S13] A. Jellinggaard, K. Grove-Rasmussen, M. H. Madsen, and J. Nygård, Phy. Rev. B **94**, 064520 (2016).
[S14] R. Deacon, Y. Tanaka, A. Oiwa, R. Sakano, K. Yoshida, K. Shibata, K. Hirakawa, and S. Tarucha, Phys. Rev. Lett. **104**, 076805 (2010).
[S15] J.-D. Pillet, P. Joyez, M. Goffman, *et al.*, Phys. Rev. B **88**, 045101 (2013).
[S16] E. J. Lee, X. Jiang, R. Aguado, C. M. Lieber, and S. De Franceschi, Phys. Rev. B **95**, 180502 (2017).
[S17] K. Grove-Rasmussen, G. Steffensen, A. Jellinggaard, M. Madsen, R. Žitko, J. Paaske, and J. Nygård, Nat. Commun. **9**, 2376 (2018).
[S18] B.-K. Kim, Y.-H. Ahn, J.-J. Kim, M.-S. Choi, M.-H. Bae, K. Kang, J. S. Lim, R. López, and N. Kim, Phys. Rev. Lett. **110**, 076803 (2013).

[S19] J. Pillet, C. Quay, P. Morfin, C. Bena, A. L. Yeyati, and P. Joyez, Nat. Phys. **6**, 965 (2010).
[S20] K. Grove-Rasmussen, H. I. Jørgensen, B. M. Andersen, J. Paaske, T. S. Jespersen, J. Nygård, K. Flensberg, and P. E. Lindelof, Phys. Rev. B **79**, 134518 (2009).
[S21] A. Eichler, M. Weiss, S. Oberholzer, C. Schönenberger, A. L. Yeyati, J. Cuevas, and A. Martín-Rodero, Phys. Rev. Lett. **99**, 126602 (2007).
[S22] E. J. Lee, X. Jiang, R. Aguado, G. Katsaros, C. M. Lieber, and S. De Franceschi, Phys. Rev. Lett. **109**, 186802 (2012).
[S23] Z. Su, A. B. Tacla, M. Hocevar, D. Car, S. R. Plissard, E. P. Bakkers, A. J. Daley, D. Pekker, and S. M. Frolov, Nat. Commun. **8**, 585 (2017).
[S24] H. Nilsson, P. Samuelsson, P. Caroff, and H. Xu, Nano Lett. **12**, 228 (2011).
[S25] Recently, replicas of subgap states were observed within the superconducting gap in single dot systems. Their origin was attributed to either additional subgap states in the leads or additional levels, or both [S51]. However, the modeling assumed a S-QD-N geometry with the N-lead strongly decoupled, which is not relevant for our case of symmetric S-leads.
[S26] As shown in the zoomed maps of Fig. 3 of the main article, at low bias a single pair of subgap states at lower $V_{sd}$ than these apparent lowest-lying subgap states does appear to cross zero bias, but the conductance of this pair is so small that it does not show in any of the maps of Fig. S3. The strongly reduced conductance of this lowest-lying pair of subgap states and their crossing of zero bias is indicative of a small density of states within the gap, too small to show in gap-spectroscopy $I - V_{sd}$ curves such as the one in Fig. S6c.
[S27] M. Deng, S. Vaitiekėnas, E. B. Hansen, J. Danon, M. Leijnse, K. Flensberg, J. Nygård, P. Krogstrup, and C. M. Marcus, Science **354**, 1557 (2016).
[S28] Y.-J. Doh, S. D. Franceschi, E. P. Bakkers, and L. P. Kouwenhoven, Nano Lett. **8**, 4098 (2008).
[S29] T. Novotný, A. Rossini, and K. Flensberg, Phys. Rev. B **72**, 224502 (2005).
[S30] A. Brunetti, A. Zazunov, A. Kundu, and R. Egger, Phys. Rev. B **88**, 144515 (2013).
[S31] K. G. Wilson, Rev. Mod. Phys. **47**, 773 (1975).
[S32] H. R. Krishna-murthy, J. W. Wilkins, and K. G. Wilson, Phys. Rev. B **21**, 1003 (1980).
[S33] K. Satori, H. Shiba, O. Sakai, and Y. Shimizu, J. Phys. Soc. Japan **61**, 3239 (1992).
[S34] O. Sakai, Y. Shimizu, H. Shiba, and K. Satori, J. Phys. Soc. Japan **62**, 3181 (1993).
[S35] T. Yoshioka and Y. Ohashi, J. Phys. Soc. Japan **67**, 1332 (1998).
[S36] T. Yoshioka and Y. Ohashi, J. Phys. Soc. Japan **69**, 1812 (2000).
[S37] W. C. Oliveira and L. N. Oliveira, Phys. Rev. B **49**, 11986 (1994).
[S38] K. Chen and C. Jayaprakash, Phys. Rev. B **52**, 14436 (1995).
[S39] V. L. Campo and L. N. Oliveira, Phys. Rev. B **72**, 104432 (2005).
[S40] R. Žitko and T. Pruschke, Phys. Rev. B **79**, 085106 (2009).
[S41] R. Žitko, M. Lee, R. López, R. Aguado, and M.-S. Choi, Phys. Rev. Lett. **105**, 116803 (2010).
[S42] R. Žitko, O. Bodensiek, and T. Pruschke, Phys. Rev. B **83**, 054512 (2011).
[S43] R. Žitko, J. S. Lim, R. Lopez, and R. Aguado, Phys. Rev. B **91**, 045441 (2015).
[S44] R. Žitko, Phys. Rev. B **91**, 165116 (2015).
[S45] K. Grove-Rasmussen, G. Steffensen, A. Jellinggaard, M. H. Madsen, R. Žitko, J. Paaske, and J. Nygård, Nat. Commun. **9**, 2376 (2018).
[S46] C. W. J. Beenakker and H. van Houten, in *Single-electron tunneling and mesoscopic devices*, edited by H. Koch and Hübbig (Springer, 1992) pp. 175–179, also available as cond-mat/0111505.
[S47] L. I. Glazman and K. A. Matveev, JETP Lett. **49**, 659 (1989).
[S48] A. V. Rozhkov, D. P. Arovas, and F. Guinea, Phys. Rev. B **64**, 233301 (2001).
[S49] A. V. Rozhkov and D. P. Arovas, Phys. Rev. Lett. **82**, 2788 (1999).
[S50] R. Delagrange, R. Weil, A. Kasumov, M. Ferrier, H. Bouchiat, and R. Deblock, Phys. Rev. B **93**, 195437 (2016).
[S51] Z. Su, A. Zarassi, J.-F. Hsu, P. San-Jose, E. Prada, R. Aguado, E. Lee, S. Gazibegovic, R. Veld, D. Car, *et al.*, arXiv preprint arXiv:1805.04289 (2018).
